# Supplementary material for: A robust approach for estimating change-points in the mean of an AR(1) process
Source: arXiv:1403.1958 source file (2015-03-03)
Supplement: Supplementary file 1 [file Appendix.tex]

\input{AppSec2.tex}

\input{AppSec3.tex}

\input{AppSec4.tex}

%%% Local Variables:
%%% mode: latex
%%% TeX-master: "Cha13.tex"
%%% End:
